# Supplementary material for: Weighted KL-Divergence for Document Ranking Model Refinement
Source: arXiv:2406.05977 source file (2024-06-10)
Supplement: Supplementary file 1 [file appendix.tex]

%\section{Details on Loss Property}
\section{ Proof of Proposition ~\ref{prop:CKLbound}}
%\section{Details on Relevance Numbers Cited and Model Implementations}
\label{sec:appendix}

%\text{Proof of Proposition ~\ref{prop:CKLbound}}.
We follow Bernoulli's inequality 
$ (1-q_i)^r \geq  1 -r q_i$. 
when $r\ge 1$ and $0\leq q_j \leq 1$. 
Considering $\ln p_i \leq 0$ and $\ln q_i \leq 0$, we have
\[
\begin{aligned}
\it{L}_{CKL} 
 = & 
\sum_{ d_j  \in \mathcal{D}^{+}} (1-q_j)^\gamma p_j \ln p_j +
\sum_{ d_i  \in \mathcal{D}^{-}} q_i^{\gamma -\beta_i} p_i \ln p_i \\
&-\sum_{ d_j  \in \mathcal{D}^{+}} (1-q_j)^\gamma p_j \ln q_j 
-\sum_{ d_i  \in \mathcal{D}^{-}} q_i^{\gamma-\beta_i}  p_i \ln q_i \\
\ge & 
\sum_{ d_j  \in \mathcal{D}^{+}} p_j \ln p_j +
\sum_{ d_i  \in \mathcal{D}^{-}} p_i \ln p_i \\
&-\sum_{ d_j  \in \mathcal{D}^{+}} (1-q_j \gamma) p_j \ln q_j 
-\sum_{ d_i  \in \mathcal{D}^{-}} q_i^{\gamma -\beta_i} p_i\ln q_i \\
= & \sum_{d_j \in \mathcal{D}^+} p_j \ln \frac{p_j} {q_j}  + \frac{\gamma}{\log e} \sum_{d_j \in \mathcal{D}^{+}}  q_j \log q_j\\
& -  \sum_{ d_i  \in D^{-}} p_i q_i^{\gamma-\beta_i}  \ln q_i 
 + \sum_{ d_i \in  \mathcal{D}^{-}} p_i  \ln p_i 
\end{aligned}
\]

The forth component in the right-hand side of the first inequality in (\ref{eq:CKLbound}) is a constant and we further derive the lower bounds for  the firs three  components as follows
\begin{itemize}
\item We apply  a known inequality: $\ln x \le x-1$ when $x$ is positive and the equality is  reached when $x=1$.
\[
\sum_{d_j \in \mathcal{D}^+} p_j \ln \frac{p_j}{q_j} 
\ge  \sum_{d_j \in \mathcal{D}^+} p_j (1- \frac{ q_j}{p_j})  \ge -1 +   \sum_{d_j \in \mathcal{D}^+}  p_j =  - \sum_{d_i \in \mathcal{D}^-}  p_i.   
\]

%The term $\sum_{i: d_{(i)} \in D^{+}} P_S^{s}(i) \log P_S^{s}(i)$ can 
%be viewed as a measure to 
\item 
%The second component quantify the entropy within positive documents.
%+ \sum_{d_i \in D^-} p_i \logc{p_i}{q_i}
The second component $ \frac{\gamma}{\log e} \sum_{d_i \in  \mathcal{D}^+} q_i \log q_i$ 
is  proportional to the entropy within positive examples.

Since function $x \log x$ is convex and  following  Jensen's inequality on a convex function,
\[
\frac{\sum_{d_j \in  \mathcal{D}^+} q_j \log q_j } {s}  \ge  
(\frac{\sum_{d_j \in  \mathcal{D}^+} q_j } {s}) 
\log (\frac{\sum_{d_j \in  \mathcal{D}^+} q_j } {s})  
\]
 where $s= |\mathcal{D}^+|$. Let $z= \sum_{d_i \in  \mathcal{D}^-} q_i$. Then
\[
\sum_{d_j \in  \mathcal{D}^+} q_j \log q_j   \ge  
( 1-z) \log (\frac{1-z } {s})  \ge -\frac{2\log e}{e}. 
\]
%where the equality is reached when $q_i  = q_j$ for any pair $d_i, d_j \in D^+$.
Expression $( 1-z) \log (\frac{1-z } {s})$ is  bounded by $-\frac{2\log e}{e}$ by computing its minimum value.
 
\item The third component $ -\sum_{d_i \in  \mathcal{D}^-} p_i q_i^{\gamma - \beta_i}  \ln q_i$, 
has minimum value 0 when $q_i=0$ or $q_i=1$ given   that
$q_i \in [0, 1]$ and   $ \gamma-\beta_i \ge 1$. 
%The chance is high that  
%minimizing the last component is 
%equivalent to minimizing $q_i$ for $\forall d_i \in D^-$. 
\end{itemize}
Adding the   above component  lower bounds together, $L_{CKL} \ge  
 \sum_{d_i \in \mathcal{D}^-} p_i (-1+ \ln p_i)  -\frac{2\gamma}{e}$.
This lower bound  is a constant because $p_i$ values from the teacher's model are constant.
\hfill $\blacksquare$

%minimising our weighted KL loss will minimizing the original KL-divergence loss, 
%plus trying to minimize the top one probabilities of negative documents. In the meanwhile, 
%it also tries to maximizing the entropy among positive documents, 
%preventing the model to favor particular positive documents over others.  

\comments{
{\bf Proof. ~\ref{prop:gradient}} 
Notice that $ \forall d_i \in \mathcal{D}^+ \cup \mathcal{D}^-,  \frac{\partial \it{L}_{KL}(i)}{\partial q_i} = -  \frac{p_i}{q_i}$.

For positive documents:

$
\begin{aligned}
\frac{\partial \it{L}_{CKL}(i)}{\partial q_i} = & -\gamma \left( 1-q_i \right)^{\gamma -1} p_i \ln \frac{p_i}{q_i} - \left(1-q_i \right)^{\gamma} \frac{p_i}{q_i}\\
 = & \frac{\partial \it{L}_{KL}(i)}{\partial q_i}  
    (1-q_i)^{\gamma -1} \times \left( \gamma q_i \ln \frac{ p_i}{q_i} + 1-q_i \right).  
\end{aligned}
$

For negative documents:

$
\begin{aligned}
\frac{\partial \it{L}_{CKL}(i)}{\partial q_i} = & (\gamma-\beta_i) \left( q_i \right)^{\gamma -\beta_i-1} p_i \ln \frac{p_i}{q_i} 
- \left(q_i \right)^{\gamma-\beta_i}  \frac{p_i}{q_i}\\
 = & \frac{\partial \it{L}_{KL}(i)}{\partial q_i}  
     q_i^{\gamma-\beta_i} \times \left( 1- (\gamma-\beta_i) \ln \frac{p_i}{q_i } \right).  
\end{aligned}
$

\hfill $\blacksquare$
}
